# Supplementary material for: NaturalConv: A Chinese Dialogue Dataset Towards Multi-turn Topic-driven Conversation
Source: arXiv:2103.02548 ancillary file (2024-11-07)
Supplement: Supplementary file 1 [file SupplementaryMaterial_AAAI-21.pdf]

# NaturalConv: A Chinese Dialogue Dataset Towards Multi-turn Topic-driven Conversation Supplementary Material

Xiaoyang Wang[1], Chen Li[1], Jianqiao Zhao, Dong Yu
Tencent AI Lab, Bellevue, WA

| |
|---|
| 舒马赫妻子首度接受采访:他为我做了一切永远不忘他的好<br>网易体育11月9日报道：舒马赫妻子科琳娜近日接受德国媒体采访，这也是自迈克尔-舒马赫在2013年发生滑雪事故以来，科琳娜首次接受专访，尽管依然不透露车王的恢复情况，不过谈到车王时，科琳娜充满了感激之情，直言自己永远不会忘记迈克尔对自己的好。2013年底舒马赫在法国滑雪时出了意外，脑部严重受伤，陷入昏迷中，而自从2014年9月回到家里接受治疗以来，关于这位F1七冠王的身体状况几乎没有被披露过，尤其科琳娜不向外界透露半个字。不过舒马赫的子女却一直活跃在人们视线中，今年20岁的米克正追随父亲的脚步，为自己的赛车生涯努力奋斗，而22岁的吉娜在赛马事业上证明了自己的运动天赋。不得不提的是，科琳娜接受专访时除了向迈克尔致敬，也表达了全家对马的热爱之情，“当我30岁的时候，我非常想要一匹马，于是迈克尔带着我去了迪拜，决定去买一匹阿拉伯马。他为我做了一切，我永远不会忘记我要感激的人，这个人就是我的丈夫迈克尔。”舒马赫和科琳娜在1995年步入婚姻殿堂，2005年两人结婚十周年的时候，舒马赫送给妻子一座位于在瑞士小镇吉林斯的牧场，而如今科琳娜在瑞士和德克萨斯拥有两个牧场，拥有40匹马。科琳娜说道：“我很高兴我有这样一个伟大的团队，让一切没有停下来，尤其当我看到女儿吉娜时，我感到无比骄傲，她已经取得了一定成就，她是那么开心，这让我感到开心。”事实上也是如此，吉娜从欧洲欧洲青年马术锦标赛起步，曾是牛仔竞技项目的世界青年女子排名第一，今年初在瑞士举办的欧洲杯上夺得一枚金牌。吉娜说道：“父亲给过我建议，他告诉我，作为车手你可以将车停在车库里，但是马需要一直照顾，即使是在星期天。”而科琳娜透露，迈克尔早就预测过，他们女儿一定会获得成功，“当我丈夫告诉我，早晚有一天吉娜会比我更出色时，我没有激动万分。我心里想的是，他是怎么得出这个结论的？我的意思是，我从早到晚都和马在一起，努力学习一切，但迈克尔强调，你确实很出色，可吉娜却能将全部精力放在马身上。”<br><br>Schumacher’s wife is interviewed for the first time: He has done everything for me and I will never forget his kindness.<br>Netease Sports reported on November 9: Schumacher’s wife Corinna was interviewed by German media recently. This is also the first time since Michael Schumacher’s skiing accident in 2013 that Corinna has been interviewed. Although the physical condition of the legendary F1 driver is still not disclosed, Corinna is full of gratitude when talking about her husband, saying that she will never forget Michael’s kindness to herself. Schumacher had an accident while skiing in France at the end of 2013. His brain was seriously injured and he was placed in a medically induced coma. Since he returned home for treatment in September 2014, little has been disclosed about the F1 seven-time champion’s physical condition. Especially, Corinna was not disclosing a word to the outside world. However, Schumacher’s children have been active in people’s eyes. Mick, 20, is following in his father’s footsteps and striving hard for his racing career. Gina, 22, has proved her athletic talent in racing. It must be mentioned that in the interview, Corinna not only paid tribute to Michael, but also expressed his family’s love for horses. “When I was 30 years old, I wanted a horse very much, so Michael took me to Dubai and decided to buy an Arab horse. He has done everything for me, and I will never forget the person I want to thank. This person is my husband Michael.” Schumacher and Corinna got married in 1995. On the 10th anniversary of their marriage in 2005, Schumacher gave his wife a ranch in the small Swiss town of Geerlings. Today, Corinna owns two ranches in Switzerland and Texas with 40 horses. Corinna said: “I am very glad that I have such a great team that everything has not stopped. Especially when I see my daughter Gina, I feel extremely proud. She has made certain achievements. She is so happy, which makes me feel happy.” As a matter of fact, Gina started with the European Youth Equestrian Championship. She was in the first place in the young women rodeo event of the world, and won a gold medal at the European Championship held in Switzerland earlier this year. Gina said: “My father gave me advice. He told me that as a driver you can park your car in the garage, but the horse needs to be taken care of all the time, even on Sundays.” Corinna revealed that Michael had long predicted that their daughter would be successful. “I was not thrilled when my husband told me that Gina would be better than me one day. What I am thinking is, how did he come to this conclusion? I mean, I stayed with the horse from morning till night and worked hard at everything, but Michael emphasized that you were really good, but Gina was able to concentrate all her energy on the horse.” |

Table 1: The news used as common topic for the dialog in Table 2.

[1]Equal contribution.

| Participant | Content of Dialogue |
|---|---|
| A | 嗨，你好呀！(Hello!) |
| B | 你好！(Hello!) |
| A | 你也在关注这个新闻吗？你平时喜欢看这类的比赛吗？(Are you also following the news? Do you usually like to read such kind of sports news?) |
| B | 不怎么喜欢，正好瞄到，反正也是在等车，打发时间。我都不认识这个人，舒马赫是做什么的呀。(I don't like it very much, just coming across when I am waiting for the bus. I don't know this person. What does Schumacher do?) |
| A | 舒马赫是一名赛车手，舒马赫对赛车充满着热情和喜爱，感觉受伤之后的他应该会再一次活跃起来吧。(Schumacher was a racing driver. He is full of enthusiasm and love for racing. He should be active again after recovering from the injury.) |
| B | 嗯嗯，报道说舒马赫在滑雪时出现意外，现在都还在昏迷，我觉得重返赛车场不怎么现实呀。(Hmmm. It says Schumacher had an accident while skiing and is still in a coma. I don't think it is very realistic for him to return to the racing circuit.) |
| A | 不过他的子女现在一直活跃在大家的眼中，米克一直为自己的赛车生涯努力着。(However, his children have been active in everyone's eyes and Mick has been working hard for his racing career.) |
| B | 是的，希望米克也能像他父亲一样在球场上发光发亮。(Yes, I hope Mick can shine like his father on the court.) |
| A | 那你平时会不会看一些赛车比赛么？(Do you usually watch the racing competitions?) |
| B | 不怎么会看，我感觉很危险啊，这是在用生命来比赛啊，以前看的时候我真的手捏一把汗啊。(I don't think so. I feel car racing is dangerous. This is a competition of life.) |
| A | 哈哈好吧，那你很惜命啊，不过这也看自己的爱好，有些人很喜欢并且有天赋。(Haha, well, then you really care about your life. But, it is also a matter of hobbies. Some people like it very much and have talent.) |
| B | 是的，我一直都很惜命，之前我中国有一个作家也是赛车手，很厉害的叫什么名字啊？(Yes, I always care about my life. I remember there is a Chinese racing driver who is also a writer. What is his name?) |
| A | 韩寒，赛车很棒啊夺过很多冠军呢。多才多艺，之前的电影《后会无期》也是韩寒执导的。(Han Han. He won lots of championships. He also directed a movie called "The Continent". He is really versatile.) |
| B | 嗯嗯，还有一个林志颖，也是很厉害的，喜欢赛车，之前看到他的赛车视频简直太佩服他了。(Yes. Jimmy Lin is also very very versatile and he likes racing too. I admired him very much when I watched his racing videos.) |
| A | 你看过林志颖的《放羊的星星》嘛？我觉得很好看。(Have you ever seen the TV series "My Lucky Star" in which Jimmy Lin was the main actor? I liked it very much.) |
| B | 看了看了，之前初中还是什么时候出来的电视剧，以前还买光碟来看呢。(Of course. It was released when I was a junior high school student. I even bought CDs to watch it again.) |
| A | 林志颖的儿子也很萌，之前参加爸爸去哪儿，我最喜欢他的儿子了。(Jimmy Lin's son is also very cute. When they attended the TV show "Where Are We Going? Dad", I liked his son the best.) |
| B | 好像林志颖的老婆是车展认识的，是他的粉丝，林志颖对她一见钟情呢。(It is said Jimmy Lin met his wife at an auto show and she was one of Jimmy Lin's fans. Jimmy Lin fell in love with her at first sight.) |
| A | 嗯嗯，现在过得很幸福啊！真的是不老男神。(Yes, they are very happy now! He is really the Prince Charming who never seems to age.) |
| B | 哈哈车来了，我先走了不聊了，拜拜！(Haha. My bus is coming. I need to go. Bye-bye!) |

Table 2: The dialog based on the news from Table 1.

谷歌发布全新Pixel Buds无线耳机售价179美元
网易科技讯10月16日消息，据国外媒体报道，当地时间周二谷歌在美国纽约召开秋季新品发布会，会上谷歌发布了全新的第二代Pixel Buds无线耳机，售价179美元，将于明年首先在美国市场上市。全新Pixel Buds无线耳机外形有白色、橙色、薄荷色和黑色四种外观颜色。耳机采用圆形设计，内侧添置一个“小尾巴”形状的稳定结构，佩戴更加牢固，且防汗防水。Pixel Buds无线耳机具备入耳自动检测功能，用户通过每个耳机都可以进行便捷的触摸控制：点击即可播放或暂停，而滑动可以调节音量大小。Pixel Buds采用独特的混音设计，在提供高质量音频的同时，能够让用户感知适量的环境声音，而自适应功能能够根据环境变化动态调整音量。每个耳机都配置两个麦克风，用户通话时能够有效抑制背景噪声，内置的语音加速计可以通过下颚骨的震动来检测语音。谷歌着重强调了Pixel Buds的远程蓝牙连接功能，其在室内的蓝牙连接距离最多可以相隔三个房间，而在室外可以达到大约110米。Pixel Buds无线耳机支持谷歌数字助理Assistant，单次充电可提供5个小时的续航时间。在充电盒的辅助下总续航时长能达到24小时。

Google releases new Pixel Buds wireless headset for $179
NetEase Science and Technology News, October 16, according to foreign media reports, Google held an autumn new product launch conference in New York, US, on Tuesday local time. At the conference, Google unveiled a brand new second-generation Pixel Buds wireless headset, priced at $179, which will be first available in the US market next year. The new Pixel Buds wireless headset comes in white, orange, mint and black. The earphones adopt a circular design, and a stable structure in the shape of a “small tail” is added to the inner side, so that the earphones can be worn more firmly and are sweatproof and waterproof. Pixel Buds wireless earphones have in-ear automatic detection function. Users can carry out convenient touch control through each earphone: click to play or pause, and slide to adjust the volume. Pixel Buds use a unique mixing design to provide high-quality audio while allowing users to perceive an appropriate amount of ambient sound. The adaptive function can dynamically adjust the volume according to changes in the environment. Each earphone is equipped with two microphones, which can effectively suppress the background noise when the user is talking. The built-in voice accelerometer can detect the voice through the vibration of the mandible bone. Google has emphasized Pixel Buds’ remote Bluetooth connection function. Its Bluetooth connection indoor distance can be up to three rooms apart, while it can reach about 110 meters outdoors. Pixel Buds wireless headset supports Google Digital Assistant and can provide 5 hours of battery life with a single charge. With the aid of the charging box, the total endurance can reach 24 hours.

Table 3: The news used as common topic for the dialog in Table 4.

| Participant | Content of Dialogue |
|---|---|
| A | 你好！(Hello!) |
| B | 你好！(Hello!) |
| A | 操场上跑步的人真多啊，大家锻炼的意识是越来越强了。(There are so many people jogging on the playground. Poeple are more and more willing to do exercise.) |
| B | 对啊，没事儿多出来运动运动挺好的。(Yes, that is right. It's good to get more exercise.) |
| A | 你现在看的这耳机看起来用的是谷歌家的新款，Pixel Buds无线耳机啊。(The earphone you are looking at now seems to be Google's new Pixel Buds wireless earphone.) |
| B | 对啊，这是朋友介绍给我的，到时候我想买一个这样的耳机，设计的还挺漂亮的。(Yes, one of my friends introduced it to me. I want to buy a headset like this. The design is quite beautiful.) |
| A | 我看它的介绍了，说能让用户稍微的感觉到环境声音，这个还挺实用的。(I saw its introduction. It says the earphone can make users feel the environmental sound slightly, which is quite practical.) |
| B | 对啊，我喜欢它的这个降噪功能，尤其是在打电话的时候，因为我习惯用耳机接电话。(Yes, I like its noise reduction function, especially when making phone calls because I am used to answering phones with headphones.) |
| A | 看来你对它很满意啊，他这蓝牙支持的距离还挺远的，差不多有三个房间。(It seems that you are very satisfied with it. Its Bluetooth function can support quite a far away distance, with almost three rooms.) |
| B | 这个我还不知道，不过这个距离已经算是相当可以的了，完全够用了。(I don't know that yet, but the distance is quite long and it's quite enough.) |
| A | 对啊，它的价格我看一百多美金，还是有点贵的，起码我是这样觉得。(Yes. Its price is more than 100 US dollars. I feel it is still a bit expensive. At least I think so.) |
| B | 这个也是一分价钱一分货，而且谷歌家的新品我觉得质量还是可以的。(Higher price usually means better product and I think the quality of Google's new product is still good.) |
| A | 我买耳机一般都习惯性买黑色的，很少买其他的颜色的。(I usually buy black earphones and seldom buy other colors.) |
| B | 我也差不多，不管是手机还是耳机也是黑色的居多，你看我现在这个也是黑色的。(I am the same. Either my cellphones or headphones are mostly black. You can see this one is also black.) |
| A | 就是觉得黑色显得更高大上一点，这应该是心里作用。(I just believe black is more luxurious. This should be a psychological effect.) |
| B | 对啊，个人习惯问题，蓝牙耳机现在越来越普遍了，比有线的方便很多。(Yes, personal habits. Bluetooth headsets are more and more common now, much more convenient than wired ones.) |
| A | 我已经好久都不用有线的耳机了，特别讨厌那个线，总是很乱。(I haven't used the wired headphones for a long time. I especially hate that cable. It's always messy.) |
| B | 收拾的时候还不好收拾，总觉得很多有线耳机会漏音。(It's not easy to tidy up. I always feel that many wired earphones could leak sound.) |
| A | 谁说不是呢，热身完了，我要开始跑步了，再见。(I agree. I finished warming up and will start jogging now. Goodbye.) |
| B | 再见！(Bye!) |

Table 4: The dialog based on the news from Table 3.

《仙剑》团队新游上线Steam 售价49元
喜欢《仙剑奇侠传》系列作品的小伙伴，应该还记得同为姚仙创造的《大富翁》系列。现在迎来了第十部作品的诞生，本次《大富翁10》也是由北软团队负责研发，将于明天（10月25日）正式上线Steam平台，大陆地区售价49元。Wegame平台将择期上线。《大富翁10》是一款经典的强手棋类游戏，玩家通过运气（投骰子）及策略（买地买卡片）赚取金钱，打败其他玩家。美术采用纯3D的Q版萌系画风。游戏模式包括：故事模式、传记模式、多人模式、联网模式。游戏玩法游戏采用回合制，初始所有玩家有一定的存款、现金、卡片。通过投骰子决定移动步数。踩中无主的地产可以购买，踩中敌人的地产需要交过路费。除了地产格，地图中还有银行、新闻、商店、魔法屋等事件格，使游戏充满变数，富有娱乐性。合理的利用手中的卡片可以主动干预随机性，增强策略性，使自己的利益最大化，为最终的胜利打下良好的基础。新模式除了传统大富翁的玩法，《大富翁10》加入了最新热斗玩法。在这新模式中地图取消了小型地产格，大多数地图格都是获取卡片的格子，玩家通过大量拾取、使用卡片，给敌人造成金钱伤害，使之破产，最终获得胜利。组队全新的组队模式，可以任意组队，队友之间可以相互加盖对方的地产，也可以制定策略集火其中一个敌人，使游戏的节奏变的更快。历代大富翁的卡片需要在地图中收集卡片点数去商店购买。要想获胜，玩家需要兼顾金钱和点数两套货币系统。《大富翁10》的卡片直接用金钱购买，取消了点数系统，相比历代节奏更快，不用度过前期的沉闷阶段，游戏一开始就更加刺激。

New video game from “Xianjian” Team goes live on Steam for 49 yuan
Friends who like the series of “Legend of Xianjian Chivalrous Man” should still remember the “Monopoly” series created by Yao Xian. Now comes the birth of its 10th generation. This “Monopoly 10” is also developed by the Beiruan team. It will be officially launched on the Steam platform tomorrow (October 25) and will be sold for 49 yuan in mainland China. The game will be launched on the Wegame platform on a later date. “Monopoly 10” is a classic hand chess game in which players earn money through luck (throwing dice) and strategy (buying land and cards) to defeat other players. The game design adopts pure 3D Q-edition style of painting. Game modes include story mode, biography mode, multiplayer mode, and online mode. The game is turn-based. Initially, all players have certain deposits, cash and cards. The number of moves is determined by throwing a dice. The players can purchase the real estate when they are on an unowned real estate, and need to pay tolls when they are other players’ real estates. In addition to the real estate grid, the map also contains event grids such as banks, news, shops and magic houses, which make the game full of variables and entertainment. Reasonable use of the cards in hand can actively interfere with randomness, enhance strategy, maximize their own interests, and lay a good foundation for the final victory. In addition to the traditional monopoly play, “Monopoly 10” has added the latest hot fight play. In this new mode, the map cancels the small real estate grids, and most map grids are grids for acquiring cards. Through a large number of cards picked up and used by the player, the opponent is financially hurt and forced into bankruptcy, and the player can then finally win. Team Formation is a brand-new team formation mode. Teams can be formed at will. Teammates can build each other’s real estates. They can also formulate strategies to focus on defeating one of the opponents first so as to speed up the game. In the previous generations of the “Monopoly” series, points need to be collected in the map to purchase cards. As a result, players need to balance two currency systems, i.e. money and points, in the previous games. In the new “Monopoly 10”, cards are purchased directly with money, eliminating the points system. Compared with the previous generations, “Monopoly 10” game pace is faster, and the game is more exciting from the beginning without going through the boring stage in the early game.

Table 5: The news used as common topic for the dialog in Table 6.

| Participant | Content of Dialogue |
| --- | --- |
| A | 你好！(Hello!) |
| B | 你好！(Hello!) |
| A | 在玩什么游戏呢？(What game are you playing?) |
| B | LOL (LOL) |
| A | 那你玩过《大富翁》么？(Have you ever played Monopoly?) |
| B | 肯定啊，那是我的童年记忆，小时候和院子里的伙伴天天放学后玩，那时候还是纸质版的。(Sure, that was my childhood memory. When I was a child, I played with my friends in the yard after school every day. At that time, it was still a paper version.) |
| A | 嗯呐，现在steam上出《大富翁10》了，还出了新模式，不错。(Well, now Steam has "Monopoly 10" and a new game mode, which is not bad.) |
| B | 是吗，我还没玩够的，多少钱啊？(Really, I haven't played enough. How much is it?) |
| A | 才49，便宜吧，而且是纯3D的Q版萌系画风，我喜欢哎。(It's only 49, cheap, and it's a pure 3D Q-edition. I like it.) |
| B | 哇哦，我得叫上我女朋友一起来玩，她最喜欢这样的画风和游戏了。(Wow, I have to call my girlfriend to play with me. She likes such painting styles and games the best.) |
| A | 羡慕，我自己一个人玩，哭唧唧。(Envy. I play alone, crying.) |
| B | 哈哈，以前还是插卡子的时候随时都是一群人玩。(Haha, I used to play with a group of people in the old times.) |
| A | 嗯呐，现在玩LOL的多了去了，都在周末开黑。(Well, I've been playing LOL a lot now and I play with friends on weekends.) |
| B | 这个游戏还是打怀旧情怀吧，不然买的人很少。(This game is still nostalgic. Otherwise, few people buy it.) |
| A | LOL免费的，而且又有电竞比赛推动发展，相比之下是小众了。(LOL is free of charge, and there is the ESports to promote its development. Monopoly is minority.) |
| B | 嗯呐，才50块钱拿来能干啥，玩玩开心吧(Well, what can we do with 50 yuan? Just have fun.) |
| A | 嘿，有时间我们一起玩啊，把你ID发给我，我加你。(Hey, let's play it together sometime. Send me your ID and I'll add you.) |
| B | 求之不得呢，OK哦。(OK. I couldn't ask for more.) |
| A | 到时候多叫些朋友一起玩吧，热闹。(Then call more friends to play together.) |
| B | 可以，再见！(Sure. Bye!) |
| A | 再见！(Bye!) |

Table 6: The dialog based on the news from Table 5.
